# Supplementary material for: Finding Groups of Cross-Correlated Features in Bi-View Data
Source: arXiv:2009.05079 source file (2024-05-13)
Supplement: Supplementary file 1 [file supp.pdf]

# Supplement to Finding Stable Groups of Cross-Correlated Features in Two Data Sets With Common Samples

Miheer Dewaskar      John Palowitch      Mark He  
Michael I. Love      Andrew B. Nobel

## Contents

|                                                                                     |           |
|-------------------------------------------------------------------------------------|-----------|
| <b>S1 Consequences of stability at the population level</b>                         | <b>2</b>  |
| <b>S2 BSP implementation details</b>                                                | <b>3</b>  |
| S2.1 Dealing with cycles and large sets . . . . .                                   | 3         |
| S2.2 Initialization heuristics for large datasets . . . . .                         | 3         |
| S2.3 Choice of $\alpha$ using half-permutation based edge-error estimates . .       | 4         |
| S2.3.1 Half-permutation . . . . .                                                   | 4         |
| S2.4 Filtering overlapping bimodules . . . . .                                      | 5         |
| S2.5 Covariate correction . . . . .                                                 | 6         |
| S2.6 Checking our p-value approximation . . . . .                                   | 6         |
| <b>S3 Simulation details</b>                                                        | <b>7</b>  |
| S3.1 Simulation model for each true bimodule . . . . .                              | 7         |
| S3.2 Results from sCCA . . . . .                                                    | 9         |
| S3.3 Performance of BSP and CONDOR on increasing sample size . .                    | 9         |
| <b>S4 GTEx results</b>                                                              | <b>11</b> |
| S4.1 Data acquisition and preprocessing . . . . .                                   | 11        |
| S4.2 Choice of false discovery parameter to BSP . . . . .                           | 11        |
| S4.3 Hardware and software stack . . . . .                                          | 11        |
| S4.4 Bimodule connectivity thresholds and network sparsity . . . . .                | 11        |
| S4.5 Connectivity of bimodules under edges from combined eQTL<br>analysis . . . . . | 13        |
| S4.6 Bimodule association networks . . . . .                                        | 13        |
| S4.7 Gene Ontology . . . . .                                                        | 13        |
| <b>S5 Climate analysis details</b>                                                  | <b>18</b> |

## S1 Consequences of stability at the population level

Here we prove that population stable bimodules are: (a) unions of connected components of the population cross-correlation network, and (b) are the Nash Equilibria of a certain two player game. First let us start with the proof of Lemma 1.

*Proof of Lemma 1.* For any subsets  $F \subseteq S$  and  $G \subseteq T$  note that  $\rho^2(F, G) > 0$  if and only if  $(F \times G) \cap E_p \neq \emptyset$ . Let  $\text{Nb}(s) \doteq \{t' \mid (s, t') \in E_p\}$  and  $\text{Nb}(t) \doteq \{s' \mid (s', t) \in E_p\}$  and denote the neighborhoods of  $s$  and  $t$  in the graph  $G_p$ . The two conditions in Definition 2.1 are equivalent to saying  $A = \cup_{t \in B} \text{Nb}(t)$  and  $B = \cup_{s \in A} \text{Nb}(s)$ , respectively. Equivalently, since  $G_p$  is a bipartite graph, the set of nodes  $H = A \cup B$  satisfies the property

$$H = \text{Nb}(H) \quad (1)$$

where  $\text{Nb}(C) \doteq \cup_{v \in C} \text{Nb}(v)$  for any subset of vertices  $C \subseteq S \cup T$ .

First, let us show that any  $H$  satisfying (1) is a union of connected components. For any  $r \in S \cup T$ , note that the connected component containing  $r$  (if  $r$  is not an isolated vertex) is defined by  $C(r) \doteq \cup_{i=0}^{\infty} C_i$  where  $C_0 = \{r\}$  and  $C_i = \text{Nb}(C_{i-1})$  for each  $i \geq 1$ . For  $r \in H$ , repeatedly applying (1) shows that  $r \in C(r) \subseteq H$  and hence

$$H = \cup_{r \in H} C(r). \quad (2)$$

Since (1) holds and  $G_p$  is a simple graph, each  $r \in H$  has at least one other neighbor. Hence  $C(r)$  is indeed a connected component for each  $r \in H$ .

Next, suppose that  $H$  is a union of connected components (hence no  $r \in H$  is isolated and (2) holds), we will show that (1) holds. Since  $\text{Nb}(C(r)) \subseteq C(r)$  for any  $r$ , if  $H$  satisfies (2) then  $\text{Nb}(H) \subseteq H$ . Further since each vertex in  $H$  is a neighbor of some vertex in its connected component, we must have  $\text{Nb}(H) \supseteq H$ . Hence (1) is satisfied and  $H$  is a stable population bimodule.  $\square$

The notion of stability in Definition 2.1 has close connections with Nash equilibrium (Nash, 1950) in game theory. To make this precise, fix an  $\epsilon > 0$ , and consider the reward function  $\Phi_\epsilon$  that for any  $A \subseteq S$  and  $B \subseteq T$  takes the value

$$\Phi_\epsilon(A, B) \doteq \sum_{s \in A} \sum_{t \in B} \rho^2(s, t) - \epsilon |A| |B|. \quad (3)$$

Consider a two player game in which player 1 chooses a subset  $A \subseteq S$ , player 2 chooses a subset  $B \subseteq T$ , and the payoff to both the players is  $\Phi_\epsilon(A, B)$ . In this setting, a pair of subsets  $(A^*, B^*)$  is called a Nash equilibrium if

$$\max_{A \subseteq S} \Phi_\epsilon(A, B^*) = \Phi_\epsilon(A^*, B^*) = \max_{B \subseteq T} \Phi_\epsilon(A^*, B).$$

The following elementary lemma shows that bimodules are the just Nash equilibria in this game.

**Lemma A.** *Let  $\delta = \min\{\rho^2(s, t) \mid s \in S, t \in T, \rho(s, t) \neq 0\}$  and  $\epsilon_0 = \delta(\max(|S|, |T|))^{-1}$ . If  $\epsilon \in (0, \epsilon_0)$  then the non-empty Nash equilibria of the game with reward function  $\Phi_\epsilon$  coincides with the family of stable population bimodules.*

*Proof.* Suppose  $0 < \epsilon < \epsilon_0$ . Fix  $A \subseteq S$  and observe that for any  $B \subseteq T$

$$\begin{aligned}\Phi_\epsilon(A, B) &= \sum_{t \in B} \sum_{s \in A} (\rho^2(s, t) - \epsilon) \\ &= \sum_{t \in B} (\rho^2(A, t) - \epsilon |A|).\end{aligned}\tag{4}$$

Since  $\epsilon |A| < \epsilon_0 |A| \leq \delta$ , for any  $t \in T$ , if  $\rho^2(A, t) > 0$  then  $\rho^2(A, t) - \epsilon |A| > 0$ . Hence the maximum over subsets  $B \subseteq T$  will be uniquely attained at

$$\arg \max_{B \subseteq T} \Phi_\epsilon(A, B) = \{t \in T \mid \rho^2(A, t) - \epsilon |A| > 0\} = \{t \in T \mid \rho^2(A, t) > 0\} \tag{5}$$

Similarly, if we fix  $A \subseteq T$ , we can show

$$\arg \max_{A \subseteq S} \Phi_\epsilon(A, B) = \{s \in S \mid \rho^2(s, B) > 0\} \tag{6}$$

Hence the pair of non-empty sets  $(A^*, B^*)$  is a Nash equilibrium if and only if

$$A^* = \{s \in S \mid \rho^2(s, B^*) > 0\} \text{ and } B^* = \{t \in T \mid \rho^2(A^*, t) > 0\}.$$

These conditions are the same as those required for  $(A^*, B^*)$  to be a population bimodule (Definition 2.1).  $\square$

## S2 BSP implementation details

### S2.1 Dealing with cycles and large sets

In practice, we do not want the sizes of the sets  $(A_k, B_k)$  in the iteration to grow too large as this slows computation, and large bimodules are difficult to interpret. Therefore the search procedure is terminated when the geometric size of  $(A_k, B_k)$  exceeds 5000. In some cases, the sequence of iterates  $(A_k, B_k)$  for  $k \in \{1, \dots, k_{max}\}$  will form a cycle of length greater than 1, and will therefore fail to reach a fixed point. To search for a nearby fixed point instead, when we encounter the cycle  $(A_k, B_k) = (A_l, B_l)$  for some  $l < k - 1$ , we set  $(A_{l+1}, B_{l+1})$  to  $(A_k \cap A_{k-1}, B_k \cap B_{k-1})$  and continue the iteration.

### S2.2 Initialization heuristics for large datasets

When  $|S| \gg |T|$ , we initialize BSP from all the features in  $T$ , but only from a subset of randomly chosen features in  $S$ . BSP sometimes discovers identical or almost-identical bimodules when starting from different initializations, often from features within the said bimodule. This problem is particularly prominent for large bimodules which may be rediscovered by thousands of initializations. Hence, to avoid some of this redundant computation, we may skip initializing BSP from features in the bimodules that have already been discovered.

## S2.3 Choice of $\alpha$ using half-permutation based edge-error estimates

To select the false discovery parameter  $\alpha$  for BSP, we estimate the *edge-error* for each value of  $\alpha$  from a pre-specified grid. The edge-error is an edge-based false discovery notion for bimodules, defined as the average fraction of erroneous essential-edges (defined in Section 3.3.1) among bimodules. Since we do not know the ground truth, we estimate the edge-error for BSP by running it on instances of the *half-permuted* dataset in which the sample labels for half of the features from each data type have been permuted. Further details are given below.

### S2.3.1 Half-permutation

Comparing results between the original and permuted data (Definition 3.1) allow us to assess the false discoveries from BSP when there are no true associations between features from  $S$  and  $T$ . However, we often expect associations between at least some variables from  $S$  and  $T$  (in fact, these are the ones that we want to find). To create a null distribution where some of pairs of features from  $S$  and  $T$  are correlated and some are not, we use the following half-permutation scheme. Let  $(\mathbb{X}, \mathbb{Y})$  denote the original data, where  $\mathbb{X}$  and  $\mathbb{Y}$  are measurements matrices for the two data types. We generate a *half-permuted* dataset  $(\tilde{\mathbb{X}}, \tilde{\mathbb{Y}})$  as follows:

1. Randomly select half the features,  $\hat{S} \subseteq S$  and  $\hat{T} \subseteq T$ , from each data type.
2. Randomly permute the rows of the submatrix of  $\mathbb{X}$  that corresponding to the columns  $\hat{S}$ , and call the resulting matrix  $\tilde{\mathbb{X}}$ . In other words, the submatrix corresponding to the features  $S \setminus \hat{S}$  is the same in  $\mathbb{X}$  and  $\tilde{\mathbb{X}}$ , while the sample labels of the submatrix of  $\tilde{\mathbb{X}}$  corresponding to features in  $\hat{S}$  have been permuted  $\tilde{\mathbb{X}}_{\hat{S}} = \mathbf{P}_1 \mathbb{X}_{\hat{S}}$  by a random permutation matrix  $\mathbf{P}_1$ .
3. Similarly, permute the rows of matrix  $\mathbb{Y}$  corresponding to the features  $\hat{T}$  using another independent permutation matrix  $\mathbf{P}_2$ . Call the resulting matrix  $\tilde{\mathbb{Y}}$ .

Note that, together, the “half-permutation” steps 2 and 3 temper the cross-correlation between pairs of features in  $\hat{S} \times T \cup S \times \hat{T}$ . Let  $\mathcal{B} = \{(A_1, B_1), (A_2, B_2) \dots (A_K, B_K)\}$  be the collection of bimodules in the half-permuted data  $(\tilde{\mathbb{X}}, \tilde{\mathbb{Y}})$ . We will assume that the collection  $\mathcal{B}$  is already filtered for overlaps (Section S2.4 below). We define the edge-error estimate for the collection  $\mathcal{B}$  as

$$\widehat{\text{edge-error}}(\mathcal{B}) = \frac{1}{|\mathcal{B}|} \sum_{(A,B) \in \mathcal{B}} \frac{\left| \text{essential-edges}(A, B) \cap (\hat{S} \times T \cup S \times \hat{T}) \right|}{\left| \text{essential-edges}(A, B) \right|}. \quad (7)$$

In practice, we generate half-permuted datasets and use the edge-error estimate (7) to choose  $\alpha$  as follows. First, we generate a pre-specified number  $N$  of

instances of the half-permuted dataset. If the covariates are present, we correct for them after the half-permutation step. Next, for each  $\alpha$  among a range of values, e.g.  $\{0.01, 0.02, \dots, 0.05\}$ , we run BSP with false discovery parameter  $\alpha$  over each of the half-permuted datasets and calculate the average edge-error (7) of the resulting collection of bimodules for that value of  $\alpha$ , averaged over all the  $N$  half-permuted instances. We can then choose an  $\alpha$  from the grid that has average edge-error smaller a pre-specified value like 0.05. Generally smaller values of  $\alpha$  tend to have smaller edge error, so we choose the largest value of  $\alpha$  from the grid that has acceptable edge error. However, we may choose a smaller value of  $\alpha$  if the bimodules are too large.

A caveat with the above procedure to select  $\alpha$  is that the edge-error estimates may be quite variable even when averaged over a large number  $N$  of half-permuted datasets. One explanation for this variability is that different  $\hat{S}$  and  $\hat{T}$  are chosen for each instance of the half-permutation. Nevertheless, if we observe variability we choose a more conservative value of  $\alpha$ . As seen in Section 4.2.1, even without access to the ground truth, we were able to keep the true edge-error under 0.05 by using the above strategy to select  $\alpha$ .

## S2.4 Filtering overlapping bimodules

Running BSP starting from different initializations may lead to a collection  $\mathcal{B} = \{(A_1^*, B_1^*), (A_2^*, B_2^*), \dots, (A_J^*, B_J^*)\}$  of  $J$ , potentially repeating and overlapping, bimodules. A typical bimodule might occur multiple times in  $\mathcal{B}$ , and distinct bimodules in  $\mathcal{B}$  might have substantial overlap. To reduce duplication, we count the *effective number* of disjoint bimodules in the collection  $\mathcal{B}$  and propose a way to select a subset of those many bimodules from  $\mathcal{B}$  that are most disjoint. Details follow.

We use the following definition  $N_e(\mathcal{B})$  of *effective number* of disjoint bimodules among the collection  $\mathcal{B}$ , adapted from Shabalin et al. (2009):

$$N_e(\mathcal{B}) \doteq \sum_{(A,B) \in \mathcal{B}} \frac{1}{|A||B|} \sum_{s \in A, t \in B} \frac{1}{C_{\mathcal{B}}(s,t)}, \quad (8)$$

where

$$C_{\mathcal{B}}(s,t) = \sum_{(A,B) \in \mathcal{B}} \mathbb{I}_{\{s \in A, t \in B\}} \quad (9)$$

is the number of bimodules that contain the pair  $(s,t)$ . As noted in Shabalin et al. (2009), the measure  $N_e$  has the property that if there were  $r$  distinct bimodules in  $\mathcal{B}$ , all disjoint when considered as collection of feature pairs, then  $N_e(\mathcal{B}) = r$ .

When there is substantial overlap between the bimodules in  $\mathcal{B}$ ,  $N_e(\mathcal{B})$  is typically smaller than  $|\mathcal{B}|$ . We can then choose  $N = \lceil N_e(\mathcal{B}) \rceil$  most distinct representative bimodules among  $\mathcal{B}$ , as follows.

**Cluster the collection of bimodules  $\mathcal{B}$  into  $N$  groups** We use hierarchical agglomerative clustering using the average linkage method (see Hastie

et al., 2009) based on the distance metric given by

$$d_J((A_1, B_1), (A_2, B_2)) = 1 - \frac{|A_1 \times B_1 \cap A_2 \times B_2|}{|A_1 \times B_1 \cup A_2 \times B_2|} \quad (10)$$

When we consider the bimodules as a collection of feature pairs, the metric  $d_J$  is simply the Jaccard distance between the bimodules.

**Select one representative bimodule from each cluster** Let  $\mathcal{C} \subseteq \mathcal{B}$  be one of the  $N$  bimodule clusters obtained in the previous step. We select a bimodule representative  $(A, B) \in \mathcal{C}$  from this cluster that maximizes the following *importance score*:

$$\text{is}_{\mathcal{C}}(A, B) = \sum_{s \in A, t \in B} \sum_{(A', B') \in \mathcal{C}} \mathbb{I}_{\{s \in A', t \in B'\}}. \quad (11)$$

The score  $\text{is}_{\mathcal{C}}(A, B)$  aggregates the importance of each feature pair within  $(A, B)$ , measured using the number of (potentially repeating) bimodules from  $\mathcal{C}$  the feature-pair was a part of. Bimodules that are larger and have more overlapping pairs will be preferred as representatives under this scheme.

## S2.5 Covariate correction

In some cases the data matrices  $[\mathbb{X}, \mathbb{Y}] \in \mathbb{R}^{n \times (p+q)}$  are accompanied by one or more covariates like sex, platform details and PEER factors that must be accounted for by removing their effects before discovering bimodules. Suppose we are given  $m$  such linearly independent covariates  $v_1, \dots, v_m \in \mathbb{R}^n$ . Here we describe how to modify BSP to remove their effects. First, we residualize each column of the original data  $[\mathbb{X}, \mathbb{Y}]$  by setting up a linear model with explanatory variables  $v_1, \dots, v_m$ . Denote the resulting matrix by  $[\mathbb{X}', \mathbb{Y}'] \in \mathbb{R}^{n \times (p+q)}$  that has columns which are projections of those of  $[\mathbb{X}, \mathbb{Y}]$  onto the subspace orthogonal to  $v_1, \dots, v_m$ . We would like to now run BSP on  $[\mathbb{X}', \mathbb{Y}']$ , however since the columns of  $[\mathbb{X}', \mathbb{Y}']$  lie on an  $n' = n - m'$  dimensional subspace, the independence assumption of p-value calculations in Section 3.3.2 would fail. However, as argued in Zhou et al. (2013), it is enough to replace the sample size  $n$  with the effective sample size of  $n'$  in the p-value calculations.

## S2.6 Checking our p-value approximation

To check the uniformity of our approximate p-value under the permutation null, we chose a bimodule  $(A, B)$  found in Section 5 and a  $t \in B$ . Then we randomly permuted the labels of gene  $t$  ( $10^5$  times), computing our p-value approximation  $\hat{p}(A, t)$  in each case. Hence we are assessing the uniformity of  $\hat{p}(A, t)$  under the permutation null distribution. The result in Figure S1 shows that the computed p-values are almost uniform but extremely small p-values show anti-conservative behavior. A potential reason for this anti-conservative behavior is that the tails

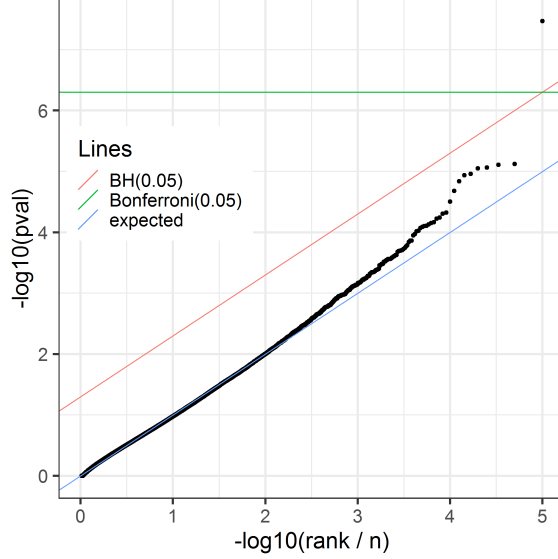

Figure S1: Assessing the accuracy of our p-value estimate  $\hat{p}(A, t)$ : We used the eQTL data from Section 5 and chose a bimodule with 24 SNPs (used as  $A$ ) and selected  $t$  to be a gene from the same bimodule. We then performed  $10^5$  random permutation of the sample labels for the gene  $t$  and repeatedly estimated  $\hat{p}(A, t)$  for each permutation after removing the effects of covariates (Appendix S2.5).

of test statistic under the permutation distribution may be heavier compared to the tails of the location-shifted Gamma distribution that we use to approximate it, since the permutation distribution is discrete distribution which explicitly depends on the exact entries of the data matrices.

## S3 Simulation details

### S3.1 Simulation model for each true bimodule

As described in Section 4, given  $\rho, \sigma \in [0, 1]$  and a binary adjacency matrix  $D \in \{0, 1\}^{|A| \times |B|}$  representing a connected bipartite graph on vertices  $A$  and  $B$  (called the regressor-graph), the variables  $(X_A, Y_A)$  for a bimodule  $(A, B)$  can be simulated as

$$X_A \sim \mathcal{N}_{|A|}(0, (1 - \rho)I + \rho U) \quad \text{and} \quad Y_B^t = D^t X_A^t + \epsilon, \quad (12)$$

where  $U$  is the matrix of all ones and  $\epsilon \sim N(0, \sigma^2)$ . The parameters  $\rho, \sigma \in [0, 1]$  and  $D$  appearing in (12) are chosen independently for each true bimodule  $(A, B)$  as follows:

1. Choose a constant  $\beta \in [0, 1]$  uniformly at random. With  $d \doteq \lceil \beta |A| \rceil$ , let  $D$  be the adjacency matrix of the  $d$ -regular bipartite connected graph

on vertex sets  $A$  and  $B$  formed by independently connecting each vertex  $t \in B$  to  $d$  randomly chosen vertices from  $A$ . If the resulting graph is not connected, set  $\beta$  to  $\beta + \Delta\beta$  where  $\Delta\beta = 0.1$  and repeat the previous step till the resulting bipartite graph is connected.

2. Randomly choose  $\rho \in [0, 1]$  and  $\eta \in [0, .8]$  subject to the constraint  $\delta \doteq 1 + \rho(d-1) \geq \eta^2 d$ . We satisfy this constraint by first uniformly generating  $\rho$  and then generating  $\eta$  uniformly from  $[0, \min(\sqrt{\delta d^{-1}}, .8)]$ .
3. Finally let  $\sigma = \frac{\sqrt{\delta(\delta - \eta^2 d)}}{\eta}$ .

The constants  $(\rho, \beta, \eta)$  in the above procedure have the following intuitive role:  $\rho$  is the intra-correlation between any two features from the set  $A$ ,  $\beta \in [0, 1]$  controls the edge density of the regressor-graph  $D$ , and  $\eta$  is the cross-correlation between features from  $B$  and adjacent features from  $A$  in the regressor-graph. The following Lemma shows that our choice of parameters indeed results in population cross-correlation of  $\eta$  between features connected by the regressor-graph:

**Lemma B.** Fix  $\rho, \eta \in [0, 1]$ ,  $a, b \in \mathbb{N}$  and  $d \in \{1, 2, \dots, a\}$  so that  $\delta \doteq 1 + \rho(d-1) \geq \eta^2 d$ . Suppose  $\mathbf{X}$  is an  $a$ -dimensional random vector with covariance matrix  $\text{Cov}(\mathbf{X}) = \rho U_a + (1 - \rho)I_a$ , where  $U_a \in \mathbb{R}^{a \times a}$  is the matrix of all ones and  $I_a \in \mathbb{R}^{a \times a}$  is the identity matrix. Next suppose  $D$  is a  $\{0, 1\}$  valued  $a \times b$  dimensional matrix that has exactly  $d$  ones in each column. Finally let  $\sigma = \sqrt{\delta(\delta - \eta^2 d)}/\eta$  and suppose the  $b$ -dimensional random vector  $\mathbf{Y}$  is given by

$$\mathbf{Y} = D^t \mathbf{X} + \boldsymbol{\epsilon}$$

where  $\boldsymbol{\epsilon}$  is another  $b$ -dimensional random vector independent of  $\mathbf{X}$  with  $\text{Cov}(\boldsymbol{\epsilon}) = \sigma^2 I_b$ . Then

$$\text{Cor}(\mathbf{X}, \mathbf{Y}) \odot D = \eta D \quad (13)$$

where  $\text{Cor}(\mathbf{X}, \mathbf{Y}) \in \mathbb{R}^{a \times b}$  is the cross-correlation matrix between random vectors  $\mathbf{X}$  and  $\mathbf{Y}$ , and  $\odot$  represents the element-wise product of matrices (i.e., the Hadamard product).

*Proof.* Since we are concerned with covariances, we can assume by mean centering that  $\mathbf{E}\mathbf{X} = \mathbf{0} \in \mathbb{R}^a$  and  $\mathbf{E}\mathbf{Y} = \mathbf{E}\boldsymbol{\epsilon} = \mathbf{0} \in \mathbb{R}^b$ . Note that  $D^t e_a = d e_b$  and  $U_a = e_a e_a^t$ , where  $e_r \doteq (1, \dots, 1)^t \in \mathbb{R}^r$  for  $r \in \{a, b\}$ . Hence using independence of  $\mathbf{X}$  and  $\boldsymbol{\epsilon}$ :

$$\begin{aligned} \text{Cov}(\mathbf{Y}) &= \mathbf{E}(\mathbf{Y}\mathbf{Y}^t) = D^t \mathbf{E}(\mathbf{X}\mathbf{X}^t) D + \mathbf{E}(\boldsymbol{\epsilon}\boldsymbol{\epsilon}^t) \\ &= D^t \text{Cov}(\mathbf{X}) D + \text{Cov}(\boldsymbol{\epsilon}) = D^t (\rho e_a e_a^t + (1 - \rho)I_a) D + \sigma^2 I_b \\ &= \rho (D^t e_a)^t (D^t e_a) + (1 - \rho) D^t D + \sigma^2 I_b \\ &= \rho d^2 e_b e_b^t + (1 - \rho) D^t D + \sigma^2 I_b \end{aligned}$$

Since all the diagonal entries of  $D^t D$  have the value  $d$ ,

$$\text{diag}[\text{Cov}(\mathbf{Y})] = (\rho d^2 + (1 - \rho)d + \sigma^2) I_b = (d\delta + \sigma^2) I_b = \left(\frac{\delta}{\eta}\right)^2 I_b \quad (14)$$



where for any square matrix  $A$ ,  $\text{diag}[A]$  denotes the diagonal matrix obtained from  $A$  by setting all the off-diagonal entries of  $A$  to 0.

We can similarly calculate the cross-covariance between  $\mathbf{X}$  and  $\mathbf{Y}$

$$\begin{aligned}\text{Cov}(\mathbf{X}, \mathbf{Y}) &= \mathbf{E}(\mathbf{XY}^t) = \mathbf{E}(\mathbf{XX}^t)D = (\rho e_a e_a^t + (1 - \rho)I_a)D \\ &= \rho d e_a e_b^t + (1 - \rho)D,\end{aligned}\tag{15}$$

and also finally the cross-correlation between  $\mathbf{X}$  and  $\mathbf{Y}$  using (15), (14) and  $\text{diag}[\text{Cov}(\mathbf{X})] = I_a$ :

$$\begin{aligned}\text{Cor}(\mathbf{X}, \mathbf{Y}) &= \text{diag}[\text{Cov}(\mathbf{X})]^{-\frac{1}{2}} \text{Cov}(\mathbf{X}, \mathbf{Y}) \text{diag}[\text{Cov}(\mathbf{Y})]^{-\frac{1}{2}} \\ &= \frac{\eta}{\delta} (\rho d e_a e_b^t + (1 - \rho)D) = \frac{\eta}{\delta} (\rho d \bar{D} + (1 - \rho + \rho d)D) \\ &= \eta D + \eta \rho d \delta^{-1} \bar{D}.\end{aligned}$$

where  $\bar{D} \doteq 1 - D$ . In particular this shows (13).  $\square$

### S3.2 Results from sCCA

We ran sCCA on the simulated dataset to search for 100 canonical covariates for a range of values of the penalty parameter  $\lambda$ . The sizes of the bimodules for various values of  $\lambda$  can be seen in Figure S2. For  $\lambda \in \{0.01, 0.02, 0.03, 0.04, .233\}$ , the first two columns of the following table show the number of true bimodules (TB) that overlapped with each detected bimodule (DB) and the edge-error of each DB averaged over all DBs. The last column shows the top 5 (or bottom 95) percentile *recall* among the true bimodules.

| $\lambda$ | # TBs that overlap with each DB | edge-error | recall of TB (95%-tile) |
|-----------|---------------------------------|------------|-------------------------|
| .01       | .97                             | .09        | .02                     |
| .02       | .96                             | .19        | .23                     |
| .03       | 1.97                            | .48        | .62                     |
| .04       | 6.47                            | .65        | .95                     |
| .23       | 281                             | .89        | 1                       |

The parameter value  $\lambda = 0.01$  has small edge-error, but poor recall. The recall improves on increasing  $\lambda$ , but the edge-error degrades.

### S3.3 Performance of BSP and CONDOR on increasing sample size

We increased that sample size of the simulation study in Section 4 to  $n = 600$ , and re-ran BSP and CONDOR with the same parameters as earlier. The average edge-error for BSP and CONDOR was 0.05 and 0.10 respectively. As seen in Figure S3, BSP and CONDOR both recall most bimodules with cross-correlation strength above 0.3, however Jaccard for BSP and CONDOR has degraded. This can be explained by noting that 25% of BSP bimodules now overlapped with two or more true bimodules compared to 6% when  $n = 200$ .

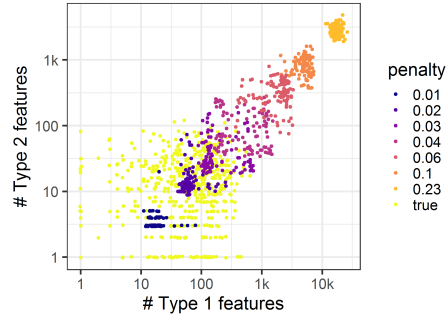

Figure S2: The sizes of sCCA bimodules for various values of the penalty parameter  $\lambda$  along with sizes of the true bimodules.

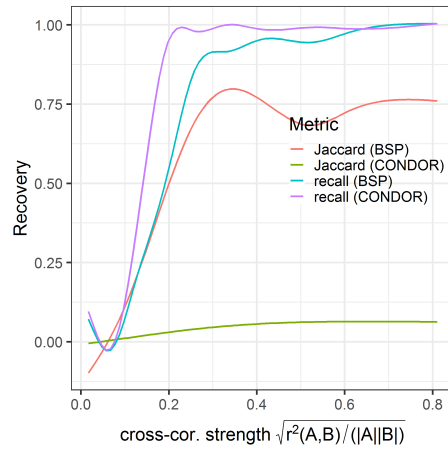

Figure S3: Average recall and Jaccard for true bimodules in the simulation with 600 samples.

## S4 GTEEx results

### S4.1 Data acquisition and preprocessing

We obtained genotype and thyroid expression data for 574 individuals from the dbGap website (accession number: phs000424.v8.p1). We directly used the filtered and normalized gene expression data and covariates provided for eQTL analysis but filtered the SNPs in the genotype data using the LD pruning software *SNPRelate* Zheng (2015). The software retained 556K autosomal SNPs with minor allele frequency above 0.1 such that all pairs of SNPs within each 500KB window of the genome had squared correlation under  $(0.7)^2$ . The latter threshold was chosen to balance the number of retained SNPs and information loss.

There were 68 covariates provided for the Thyroid tissue consisting of the top 5 genotype principle components; 60 PEER covariates, and 3 additional covariates for sequencing platform, sequencing protocol, and sex. We accounted for these covariates by the modification to BSP mentioned in Appendix S2.5.

### S4.2 Choice of false discovery parameter to BSP

We chose the false discover parameter  $\alpha$  for BSP from the grid  $\{0.01, 0.02, 0.03, 0.04, 0.05\}$  by finding the largest  $\alpha$  that kept the average edge-error estimates based on  $N = 5$  half-permutations under 0.05 (see Appendix S2.3). However our error estimates were variable as we obtained  $\alpha = 0.05$  in one instance and  $\alpha = 0.03$  in another. We conservatively chose  $\alpha = 0.03$ .

### S4.3 Hardware and software stack

The various methods used in this analysis were run on a dedicated computer that had Intel (R) Xeon (R) E5-2640 CPU with 20 parallel cores at 2.50 Hz base frequency, and a 512 GB random access memory along with L1, L2 and L3 caches of sizes 1.3, 5 and 50 MB respectively. The computer ran Windows server 2012 R2 operating system and we used the Microsoft R Open 3.5.3 software to perform most of our analysis, since it has multi-core implementations of linear algebra routines.

### S4.4 Bimodule connectivity thresholds and network sparsity

Figure S4 shows two network statistics for bimodules found by BSP – connectivity threshold and tree-multiplicity. All bimodules have tree multiplicity under 10. This shows that the association network for large bimodules, particularly having low connectivity-thresholds, is sparse.

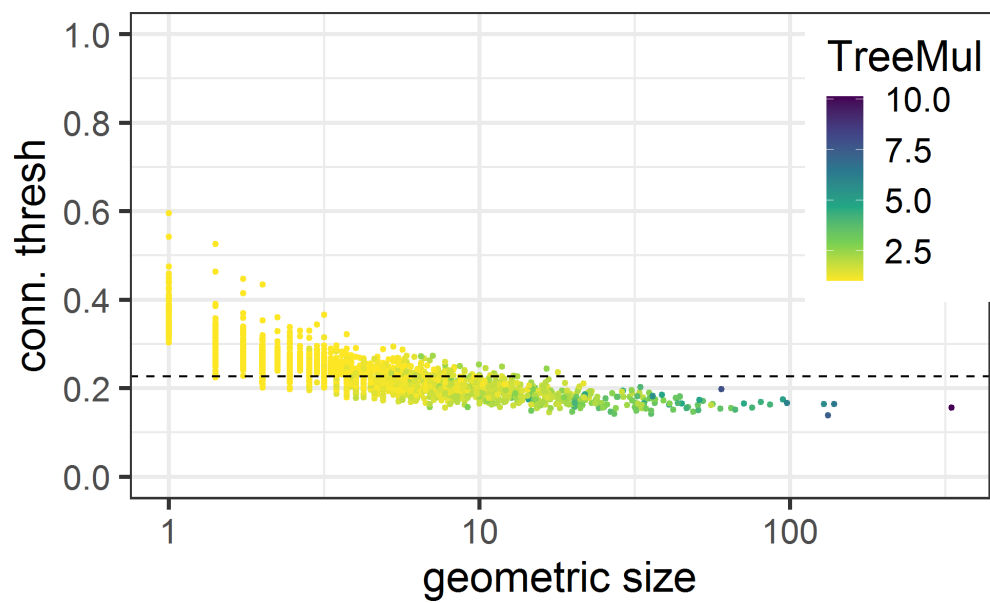

Figure S4: Connectivity-threshold and tree-multiplicity for BSP bimodules compared to their geometric size. The horizontal dotted line represents the threshold obtained from standard trans-analysis.

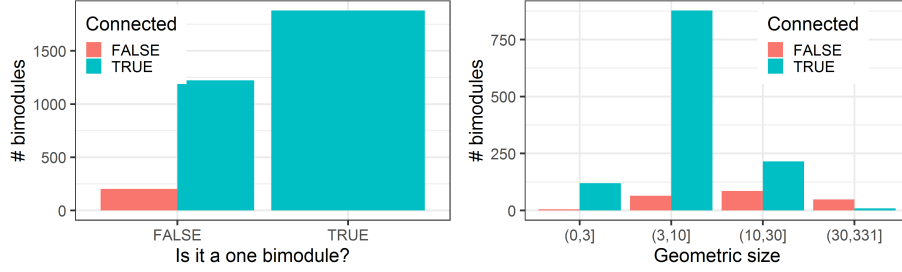

Figure S5: Connectivity of BSP bimodules under combined edges from *cis*-eQTL and *trans*-eQTL analysis. Left: the number of bimodules that are connected and are *one bimodules*, i.e. have one gene or one SNP. Right: Among bimodules having two or more genes and SNPs (i.e. are not one bimodules), the connectivity and geometric size of the bimodules.

#### S4.5 Connectivity of bimodules under edges from combined eQTL analysis

Here we examine which bimodules are connected under the combined edges from *cis*-eQTL and *trans*-eQTL analysis, based on geometric size of the bimodule. Figure S5 (left) shows that all the bimodules that have either one gene or one SNP are connected. Hence, these bimodules could have been recovered using standard eQTL analysis. On the other hand if we restrict to bimodules with two or more genes and SNPs, we see that (Figure S5; right) the fraction of connected bimodules tends to decrease as the geometric size of the bimodules increases.

#### S4.6 Bimodule association networks

See the plots in Figure S6.

#### S4.7 Gene Ontology

18 out of the 145 BSP gene sets, and 1 out of the 5 CONDOR gene sets that we considered had significant overlap with GO categories. Among the 40 GO terms detected by the CONDOR, 27 terms were also found among the 135 terms detected by BSP. The GO terms that were discovered for the two methods did not seem specific to thyroid, the tissue under investigation. Complete list of the GO terms for the two methods is as follows. Significant GO terms for BSP:

|   | GO.ID      | Term                                        | bimod. |
|---|------------|---------------------------------------------|--------|
| 1 | GO:0060333 | interferon-gamma-mediated signaling path... | 1      |
| 2 | GO:0002478 | antigen processing and presentation of e... | 1      |
| 3 | GO:0019884 | antigen processing and presentation of e... | 1      |
| 4 | GO:0048002 | antigen processing and presentation of p... | 1      |

|    |            |                                             |   |
|----|------------|---------------------------------------------|---|
| 5  | GO:0019882 | antigen processing and presentation         | 1 |
| 6  | GO:0071346 | cellular response to interferon-gamma       | 1 |
| 7  | GO:0034341 | response to interferon-gamma                | 1 |
| 8  | GO:0019886 | antigen processing and presentation of e... | 1 |
| 9  | GO:0002495 | antigen processing and presentation of p... | 1 |
| 10 | GO:0002504 | antigen processing and presentation of p... | 1 |
| 11 | GO:0045087 | innate immune response                      | 1 |
| 12 | GO:0050776 | regulation of immune response               | 1 |
| 13 | GO:0006952 | defense response                            | 1 |
| 14 | GO:0031295 | T cell costimulation                        | 1 |
| 15 | GO:0031294 | lymphocyte costimulation                    | 1 |
| 16 | GO:0050852 | T cell receptor signaling pathway           | 1 |
| 17 | GO:0002768 | immune response-regulating cell surface ... | 1 |
| 18 | GO:0002764 | immune response-regulating signaling pat... | 1 |
| 19 | GO:0050851 | antigen receptor-mediated signaling path... | 1 |
| 20 | GO:0002682 | regulation of immune system process         | 1 |
| 21 | GO:0022409 | positive regulation of cell-cell adhesio... | 1 |
| 22 | GO:0002253 | activation of immune response               | 1 |
| 23 | GO:0002429 | immune response-activating cell surface ... | 1 |
| 24 | GO:0006950 | response to stress                          | 1 |
| 25 | GO:0006955 | immune response                             | 1 |
| 26 | GO:0019221 | cytokine-mediated signaling pathway         | 1 |
| 27 | GO:0002757 | immune response-activating signal transd... | 1 |
| 28 | GO:0050870 | positive regulation of T cell activation    | 1 |
| 29 | GO:0002479 | antigen processing and presentation of e... | 1 |
| 30 | GO:1903039 | positive regulation of leukocyte cell-ce... | 1 |
| 31 | GO:0042590 | antigen processing and presentation of e... | 1 |
| 32 | GO:0045806 | negative regulation of endocytosis          | 2 |
| 33 | GO:0050911 | detection of chemical stimulus involved ... | 3 |
| 34 | GO:0007608 | sensory perception of smell                 | 3 |
| 35 | GO:0050907 | detection of chemical stimulus involved ... | 3 |
| 36 | GO:0009593 | detection of chemical stimulus              | 3 |
| 37 | GO:0007606 | sensory perception of chemical stimulus     | 3 |
| 38 | GO:0035459 | cargo loading into vesicle                  | 3 |
| 39 | GO:0050906 | detection of stimulus involved in sensor... | 3 |
| 40 | GO:0000038 | very long-chain fatty acid metabolic pro... | 4 |
| 41 | GO:0006732 | coenzyme metabolic process                  | 4 |
| 42 | GO:0006417 | regulation of translation                   | 5 |
| 43 | GO:0034248 | regulation of cellular amide metabolic p... | 5 |
| 44 | GO:0010608 | posttranscriptional regulation of gene e... | 5 |
| 45 | GO:0046597 | negative regulation of viral entry into ... | 6 |
| 46 | GO:0035455 | response to interferon-alpha                | 6 |
| 47 | GO:0035456 | response to interferon-beta                 | 6 |
| 48 | GO:0046596 | regulation of viral entry into host cell    | 6 |
| 49 | GO:0045071 | negative regulation of viral genome repl... | 6 |
| 50 | GO:1903901 | negative regulation of viral life cycle     | 6 |

|    |            |                                             |   |
|----|------------|---------------------------------------------|---|
| 51 | GO:0060337 | type I interferon signaling pathway         | 6 |
| 52 | GO:0071357 | cellular response to type I interferon      | 6 |
| 53 | GO:0034340 | response to type I interferon               | 6 |
| 54 | GO:0045069 | regulation of viral genome replication      | 6 |
| 55 | GO:0048525 | negative regulation of viral process        | 6 |
| 56 | GO:0019079 | viral genome replication                    | 6 |
| 57 | GO:0046718 | viral entry into host cell                  | 6 |
| 58 | GO:1903900 | regulation of viral life cycle              | 6 |
| 59 | GO:0030260 | entry into host cell                        | 6 |
| 60 | GO:0044409 | entry into host                             | 6 |
| 61 | GO:0051806 | entry into cell of other organism involv... | 6 |
| 62 | GO:0051828 | entry into other organism involved in sy... | 6 |
| 63 | GO:0043901 | negative regulation of multi-organism pr... | 6 |
| 64 | GO:0034341 | response to interferon-gamma                | 6 |
| 65 | GO:0050792 | regulation of viral process                 | 6 |
| 66 | GO:0051607 | defense response to virus                   | 6 |
| 67 | GO:0051701 | interaction with host                       | 6 |
| 68 | GO:0043903 | regulation of symbiosis, encompassing mu... | 6 |
| 69 | GO:0009615 | response to virus                           | 6 |
| 70 | GO:0051225 | spindle assembly                            | 7 |
| 71 | GO:0007030 | Golgi organization                          | 7 |
| 72 | GO:0007051 | spindle organization                        | 7 |
| 73 | GO:0010256 | endomembrane system organization            | 7 |
| 74 | GO:0000226 | microtubule cytoskeleton organization       | 7 |
| 75 | GO:0007017 | microtubule-based process                   | 7 |
| 76 | GO:0070925 | organelle assembly                          | 7 |
| 77 | GO:0007010 | cytoskeleton organization                   | 7 |
| 78 | GO:0007156 | homophilic cell adhesion via plasma memb... | 8 |
| 79 | GO:0098742 | cell-cell adhesion via plasma-membrane a... | 8 |
| 80 | GO:0098609 | cell-cell adhesion                          | 8 |
| 81 | GO:0007155 | cell adhesion                               | 8 |
| 82 | GO:0022610 | biological adhesion                         | 8 |
| 83 | GO:0007416 | synapse assembly                            | 8 |
| 84 | GO:0007267 | cell-cell signaling                         | 8 |
| 85 | GO:0006355 | regulation of transcription, DNA-templat... | 9 |
| 86 | GO:1903506 | regulation of nucleic acid-templated tra... | 9 |
| 87 | GO:2001141 | regulation of RNA biosynthetic process      | 9 |
| 88 | GO:0006351 | transcription, DNA-templated                | 9 |
| 89 | GO:0097659 | nucleic acid-templated transcription        | 9 |
| 90 | GO:0032774 | RNA biosynthetic process                    | 9 |
| 91 | GO:0051252 | regulation of RNA metabolic process         | 9 |
| 92 | GO:2000112 | regulation of cellular macromolecule bio... | 9 |
| 93 | GO:0010556 | regulation of macromolecule biosynthetic... | 9 |
| 94 | GO:0019219 | regulation of nucleobase-containing comp... | 9 |
| 95 | GO:0031326 | regulation of cellular biosynthetic proc... | 9 |
| 96 | GO:0034654 | nucleobase-containing compound biosynthe... | 9 |

|     |            |                                             |    |
|-----|------------|---------------------------------------------|----|
| 97  | GO:0009889 | regulation of biosynthetic process          | 9  |
| 98  | GO:0018130 | heterocycle biosynthetic process            | 9  |
| 99  | GO:0019438 | aromatic compound biosynthetic process      | 9  |
| 100 | GO:0010468 | regulation of gene expression               | 9  |
| 101 | GO:1901362 | organic cyclic compound biosynthetic pro... | 9  |
| 102 | GO:0016070 | RNA metabolic process                       | 9  |
| 103 | GO:0001580 | detection of chemical stimulus involved ... | 10 |
| 104 | GO:0050912 | detection of chemical stimulus involved ... | 10 |
| 105 | GO:0050913 | sensory perception of bitter taste          | 10 |
| 106 | GO:0050909 | sensory perception of taste                 | 10 |
| 107 | GO:0050907 | detection of chemical stimulus involved ... | 10 |
| 108 | GO:0009593 | detection of chemical stimulus              | 10 |
| 109 | GO:0007606 | sensory perception of chemical stimulus     | 10 |
| 110 | GO:0050906 | detection of stimulus involved in sensor... | 10 |
| 111 | GO:0007600 | sensory perception                          | 10 |
| 112 | GO:0051606 | detection of stimulus                       | 10 |
| 113 | GO:0050877 | nervous system process                      | 10 |
| 114 | GO:0003008 | system process                              | 10 |
| 115 | GO:0007186 | G-protein coupled receptor signaling pat... | 10 |
| 116 | GO:0006355 | regulation of transcription, DNA-templat... | 11 |
| 117 | GO:1903506 | regulation of nucleic acid-templated tra... | 11 |
| 118 | GO:2001141 | regulation of RNA biosynthetic process      | 11 |
| 119 | GO:0006351 | transcription, DNA-templated                | 11 |
| 120 | GO:0097659 | nucleic acid-templated transcription        | 11 |
| 121 | GO:0032774 | RNA biosynthetic process                    | 11 |
| 122 | GO:0051252 | regulation of RNA metabolic process         | 11 |
| 123 | GO:2000112 | regulation of cellular macromolecule bio... | 11 |
| 124 | GO:0010556 | regulation of macromolecule biosynthetic... | 11 |
| 125 | GO:0019219 | regulation of nucleobase-containing comp... | 11 |
| 126 | GO:0031326 | regulation of cellular biosynthetic proc... | 11 |
| 127 | GO:0034654 | nucleobase-containing compound biosynthe... | 11 |
| 128 | GO:0009889 | regulation of biosynthetic process          | 11 |
| 129 | GO:0018130 | heterocycle biosynthetic process            | 11 |
| 130 | GO:0019438 | aromatic compound biosynthetic process      | 11 |
| 131 | GO:0010468 | regulation of gene expression               | 11 |
| 132 | GO:1901362 | organic cyclic compound biosynthetic pro... | 11 |
| 133 | GO:0016070 | RNA metabolic process                       | 11 |
| 134 | GO:1901685 | glutathione derivative metabolic process    | 12 |
| 135 | GO:1901687 | glutathione derivative biosynthetic proc... | 12 |
| 136 | GO:0006749 | glutathione metabolic process               | 12 |
| 137 | GO:0042178 | xenobiotic catabolic process                | 12 |
| 138 | GO:0042537 | benzene-containing compound metabolic pr... | 12 |
| 139 | GO:0006575 | cellular modified amino acid metabolic p... | 12 |
| 140 | GO:0044272 | sulfur compound biosynthetic process        | 12 |
| 141 | GO:0046854 | phosphatidylinositol phosphorylation        | 13 |
| 142 | GO:0046834 | lipid phosphorylation                       | 13 |



|     |            |                                             |    |
|-----|------------|---------------------------------------------|----|
| 143 | GO:0048015 | phosphatidylinositol-mediated signaling     | 13 |
| 144 | GO:0048017 | inositol lipid-mediated signaling           | 13 |
| 145 | GO:0006882 | cellular zinc ion homeostasis               | 14 |
| 146 | GO:0055069 | zinc ion homeostasis                        | 14 |
| 147 | GO:0010273 | detoxification of copper ion                | 14 |
| 148 | GO:1990169 | stress response to copper ion               | 14 |
| 149 | GO:0061687 | detoxification of inorganic compound        | 14 |
| 150 | GO:0097501 | stress response to metal ion                | 14 |
| 151 | GO:0071294 | cellular response to zinc ion               | 14 |
| 152 | GO:0071280 | cellular response to copper ion             | 14 |
| 153 | GO:0046916 | cellular transition metal ion homeostasi... | 14 |
| 154 | GO:0071276 | cellular response to cadmium ion            | 14 |
| 155 | GO:0046688 | response to copper ion                      | 14 |
| 156 | GO:0055076 | transition metal ion homeostasis            | 14 |
| 157 | GO:0072488 | ammonium transmembrane transport            | 15 |
| 158 | GO:0006089 | lactate metabolic process                   | 16 |
| 159 | GO:0006882 | cellular zinc ion homeostasis               | 17 |
| 160 | GO:0055069 | zinc ion homeostasis                        | 17 |
| 161 | GO:0006882 | cellular zinc ion homeostasis               | 18 |
| 162 | GO:0055069 | zinc ion homeostasis                        | 18 |

#### Significant GO terms for CONDOR

|    | GO.ID      | Term                                        | bimod |
|----|------------|---------------------------------------------|-------|
| 1  | GO:0050852 | T cell receptor signaling pathway           | 1     |
| 2  | GO:0050851 | antigen receptor-mediated signaling path... | 1     |
| 3  | GO:0006355 | regulation of transcription, DNA-templat... | 1     |
| 4  | GO:1903506 | regulation of nucleic acid-templated tra... | 1     |
| 5  | GO:2001141 | regulation of RNA biosynthetic process      | 1     |
| 6  | GO:0060333 | interferon-gamma-mediated signaling path... | 2     |
| 7  | GO:0002478 | antigen processing and presentation of e... | 3     |
| 8  | GO:0019884 | antigen processing and presentation of e... | 3     |
| 9  | GO:0048002 | antigen processing and presentation of p... | 3     |
| 10 | GO:0019886 | antigen processing and presentation of e... | 3     |
| 11 | GO:0002495 | antigen processing and presentation of p... | 3     |
| 12 | GO:0002504 | antigen processing and presentation of p... | 3     |
| 13 | GO:0019882 | antigen processing and presentation         | 3     |
| 14 | GO:0031295 | T cell costimulation                        | 3     |
| 15 | GO:0031294 | lymphocyte costimulation                    | 3     |
| 16 | GO:0060333 | interferon-gamma-mediated signaling path... | 3     |
| 17 | GO:0050852 | T cell receptor signaling pathway           | 3     |
| 18 | GO:0050870 | positive regulation of T cell activation    | 3     |
| 19 | GO:1903039 | positive regulation of leukocyte cell-ce... | 3     |
| 20 | GO:0050778 | positive regulation of immune response      | 3     |
| 21 | GO:0002253 | activation of immune response               | 3     |

|    |            |                                             |   |
|----|------------|---------------------------------------------|---|
| 22 | GO:0050851 | antigen receptor-mediated signaling path... | 3 |
| 23 | GO:0022409 | positive regulation of cell-cell adhesio... | 3 |
| 24 | GO:0071346 | cellular response to interferon-gamma       | 3 |
| 25 | GO:0051251 | positive regulation of lymphocyte activa... | 3 |
| 26 | GO:1903037 | regulation of leukocyte cell-cell adhesi... | 3 |
| 27 | GO:0034341 | response to interferon-gamma                | 3 |
| 28 | GO:0002696 | positive regulation of leukocyte activat... | 3 |
| 29 | GO:0050863 | regulation of T cell activation             | 3 |
| 30 | GO:0050867 | positive regulation of cell activation      | 3 |
| 31 | GO:0007159 | leukocyte cell-cell adhesion                | 3 |
| 32 | GO:0050776 | regulation of immune response               | 3 |
| 33 | GO:0002429 | immune response-activating cell surface ... | 3 |
| 34 | GO:0002684 | positive regulation of immune system pro... | 3 |
| 35 | GO:0006955 | immune response                             | 3 |
| 36 | GO:0022407 | regulation of cell-cell adhesion            | 3 |
| 37 | GO:0045087 | innate immune response                      | 3 |
| 38 | GO:0002768 | immune response-regulating cell surface ... | 3 |
| 39 | GO:0045785 | positive regulation of cell adhesion        | 3 |
| 40 | GO:0002455 | humoral immune response mediated by circ... | 3 |
| 41 | GO:0051249 | regulation of lymphocyte activation         | 3 |
| 42 | GO:0019221 | cytokine-mediated signaling pathway         | 3 |
| 43 | GO:0042110 | T cell activation                           | 3 |

---

## S5 Climate analysis details

Figure S7 shows the edge-error estimates we used to choose  $\alpha$ . Table S3 show a summary of cross-correlations for each precipitation pixel from the two BSP bimodules.

## References

- John F. Nash. Equilibrium points in n-person games. *Proceedings of the National Academy of Sciences*, 36(1):48–49, 1950. ISSN 0027-8424. doi: 10.1073/pnas.36.1.48. URL <https://www.pnas.org/content/36/1/48>.
- Andrey A Shabalin, Victor J Weigman, Charles M Perou, Andrew B Nobel, et al. Finding large average submatrices in high dimensional data. *The Annals of Applied Statistics*, 3(3):985–1012, 2009.
- Trevor Hastie, Robert Tibshirani, and Jerome Friedman. *The elements of statistical learning: data mining, inference, and prediction*. Springer Science & Business Media, 2009.
- Yi-Hui Zhou, William T Barry, and Fred A Wright. Empirical pathway analysis, without permutation. *Biostatistics*, 14(3):573–585, 2013.

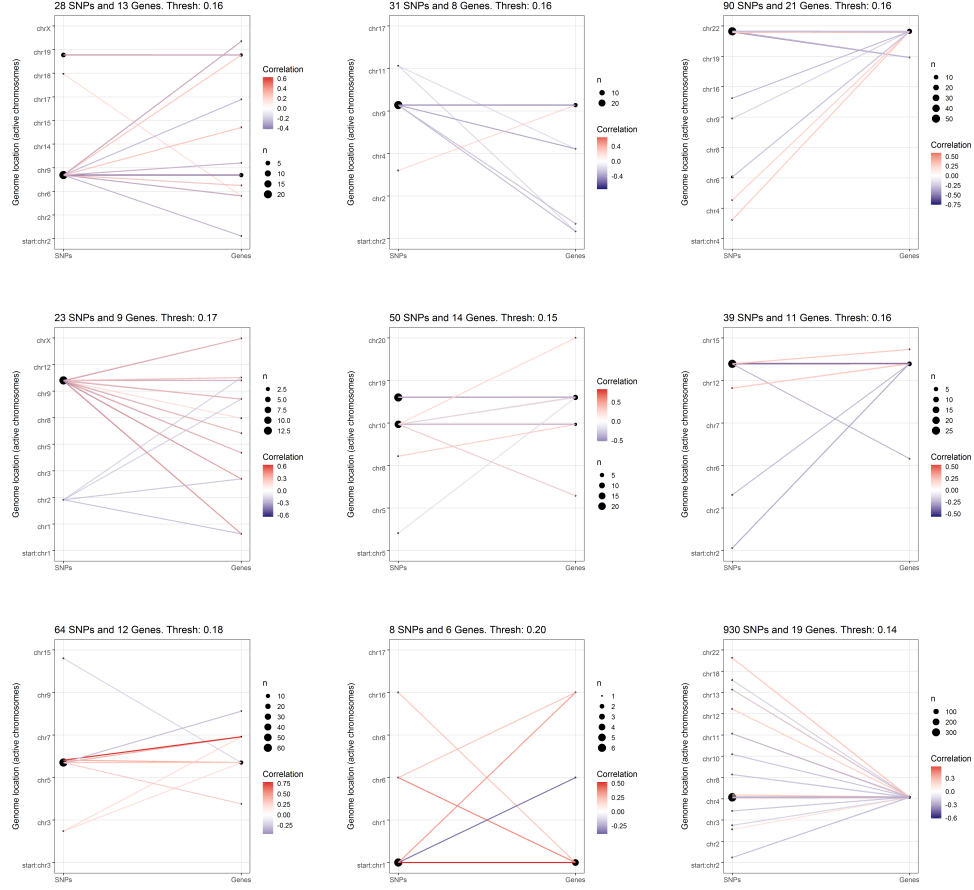

Figure S6: Out of 31 BSP bimodules that had genes on 3 or more chromosomes and SNPs on 2 or more chromosomes, we selected 9 bimodules that looked interesting. The bipartite graph for each bimodule is formed out of the essential edges (Section 5.3.3).

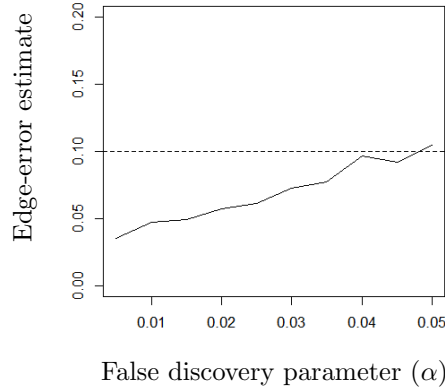

Figure S7: Average edge-error estimates for BSP results for the climate data based on 100 half-permutations (Section S2.3.1) for  $\alpha$  ranging from 0.01 to 0.05. The edge-error estimates exceed 0.05 for the first time at  $\alpha = 0.045$ .

|          | <i>P</i> Pixel | Mean | SD   |
|----------|----------------|------|------|
| <i>A</i> | 1              | 0.28 | 0.07 |
|          | 2              | 0.27 | 0.06 |
|          | 3              | 0.28 | 0.08 |
|          | 4              | 0.27 | 0.08 |
|          | 5              | 0.31 | 0.06 |
|          | 6              | 0.30 | 0.08 |
|          | <i>P</i> Pixel | Mean | SD   |
| <i>B</i> | 1              | 0.31 | 0.04 |
|          | 2              | 0.35 | 0.03 |
|          | 3              | 0.29 | 0.04 |

Table S3: Summary of the cross-correlations for each precipitation ( $P$ ) pixel in the two BSP bimodules *A* and *B* from the climate data. Each entry shows the mean and standard deviation of the cross-correlations of each  $P$  in the bimodule with other  $T$  pixels in the same bimodule. Results show that all of the cross-correlations tend to be strong and positive.

Xiuwen Zheng. *A Tutorial for the R/Bioconductor Package SNPRelate*, 2015.
